# Supplementary material for: Low-Energy Polymeric Phases of Alanates
Source: arXiv:1211.0718 source file (2013-03-27)
Supplement: Supplementary file 1 [file supplement_alanate.pdf]

# Supplemental Material: Low-Energy Polymeric Phases of Alanates

Tran Doan Huan,[1] Maximilian Amsler,[1] Miguel A. L. Marques,[2]
Silvana Botti,[2] Alexander Willand,[1] and Stefan Goedecker[1]

[1] *Department of Physics, Universität Basel, Klingelbergstrasse 82, 4056 Basel, Switzerland*
[2] *Université de Lyon, F-69000 Lyon, France and LPMCN, CNRS, UMR 5586, Université Lyon 1, F-69622 Villeurbanne, France*

(Dated: October 29, 2012)

TABLE I: Crystallographic information of the polymeric phases of $LiAlH_4$, $NaAlH_4$, $KAlH_4$, $Mg(AlH_4)_2$, $Ca(AlH_4)_2$, and $Sr(AlH_4)_2$ reported in Table 1 of the text. Three polymeric phases of $LiAlH_4$ were taken from Amsler *et. al*, Phys. Rev. Lett. **108**, 205505 (2012). The reference structure of $Sr(AlH_4)_2$, which is isolated, is also given. For each structure, cell parameters are given while for each atom, the Wyckoff site and the coordinates ($x$, $y$, and $z$) are given.

| | |
|---|---|
| **Lithium alanate $LiAlH_4$** | |
| $P2_1/c$ (14) | $a = 5.16$Å, $b = 4.27$Å, $c = 5.09$Å |
| | $\alpha = 90°$, $\beta = 66.84°$, $\gamma = 90°$ |
| Li | (2b) (0.50000, 0.00000, 0.00000) |
| Al | (2c) (0.00000, 0.00000, 0.50000) |
| H | (4e) (0.13078, 0.27635, -0.31938) |
| H | (4e) (-0.31571, 0.17575, -0.37421) |
| $P2_1$ (4) | $a = 8.95$Å, $b = 4.26$Å, $c = 5.65$Å |
| | $\alpha = 90°$, $\beta = 72.14°$, $\gamma = 90°$ |
| Li | (2a) (0.37457, -0.28106, -0.06011) |
| Li | (2a) (-0.12448, -0.28716, 0.17209) |
| Al | (2a) (0.12440, 0.21972, 0.31117) |
| Al | (2a) (-0.37431, 0.21172, -0.44005) |
| H | (2a) (0.22067, 0.41391, 0.05002) |
| H | (2a) (-0.27624, 0.43397, -0.26465) |
| H | (2a) (-0.02773, -0.47771, -0.14545) |
| H | (2a) (-0.47225, -0.00521, 0.38450) |
| H | (2a) (-0.22202, -0.08255, -0.49578) |
| H | (2a) (-0.46952, 0.03961, -0.17022) |
| H | (2a) (0.27794, -0.11397, -0.29145) |
| H | (2a) (-0.02591, -0.48353, 0.40997) |
| $Pnc2$ (30) | $a = 4.75$Å, $b = 4.22$Å, $c = 5.10$Å |
| | $\alpha = \beta = \gamma = 90°$ |
| Li | (2b) (0.50000, 0.00000, 0.33423) |
| Al | (2a) (0.00000, 0.00000, -0.35590) |
| H | (4c) (0.14407, 0.25389, -0.11765) |
| H | (4c) (-0.30273, 0.20155, -0.38289) |
| **Sodium alanate $NaAlH_4$** | |
| $C2/m$ (12) | $a = 15.24$Å, $b = 3.50$Å, $c = 5.39$Å |
| | $\alpha = 90°$, $\beta = 107.56°$, $\gamma = 90°$ |
| Na | (4i) (-0.34347, 0.00000, -0.24813) |
| Al | (4i) (-0.08953, 0.00000, -0.16280) |
| H | (4i) (0.14076, 0.00000, 0.48462) |
| H | (4i) (-0.02391, 0.00000, 0.18320) |
| H | (4i) (-0.18490, 0.00000, -0.06296) |
| H | (4i) (0.41686, 0.00000, -0.14113) |
| $P\bar{1}$ (2) | $a = 5.11$Å, $b = 6.60$Å, $c = 4.43$Å |
| | $\alpha = 88.82°$, $\beta = 90.50°$, $\gamma = 111.19°$ |
| Na | (2i) (0.38439, -0.29274, -0.15606) |
| Al | (2i) (-0.01100, -0.12960, 0.25799) |
| H | (2i) (0.19398, -0.03107, -0.07664) |
| H | (2i) (0.21437, -0.24151, 0.38794) |
| H | (2i) (-0.19577, -0.13495, -0.41092) |

to be continued ..

**TABLE I – continued from previous page**

| | |
|---|---|
| H | (2i) (-0.24437, -0.34895, 0.09836) |
| $C2$ (5) | $a = 10.54$Å, $b = 6.52$Å, $c = 4.42$Å |
| | $\alpha = 90°$, $\beta = 112.70°$, $\gamma = 90°$ |
| Na | (4c) (0.20281, 0.30470, -0.39229) |
| Al | (2b) (0.00000, -0.16513, 0.50000) |
| Al | (2a) (0.00000, -0.42516, 0.00000) |
| H | (4c) (-0.40240, 0.11790, 0.42446) |
| H | (4c) (-0.38550, 0.49384, 0.45075) |
| H | (4c) (0.40619, 0.28509, 0.08137) |
| H | (4c) (0.11308, 0.40560, -0.03366) |
| **Potassium alanate $KAlH_4$** | |
| $P\bar{1}$ (2) | $a = 6.70$Å, $b = 4.45$Å, $c = 6.06$Å |
| | $\alpha = 92.75°, \beta = 68.97°, \gamma = 72.32°$ |
| K | (2i) (-0.34460, -0.40015, -0.31700) |
| Al | (2i) (-0.12691, -0.18304, 0.10928) |
| H | (2i) (0.15276, -0.15067, 0.04133) |
| H | (2i) (-0.37153, -0.22773, 0.12201) |
| H | (2i) (0.02012, -0.44186, -0.18993) |
| H | (2i) (-0.23324, 0.03462, 0.38658) |
| $Ama2$ (40) | $a = 7.82$Å, $b = 15.17$Å, $c = 5.67$Å |
| | $\alpha = \beta = \gamma = 90.00°$ |
| K | (4b) (0.25000, 0.07042, -0.00532) |
| K | (4b) (0.25000, 0.27536, -0.49053) |
| Al | (8c) (0.41240, 0.39549, 0.02217) |
| H | (4b) (0.25000, 0.30881, -0.00499) |
| H | (8c) (0.47811, 0.13427, 0.28331) |
| H | (8c) (0.02473, -0.34359, 0.23133) |
| H | (4a) (0.00000, 0.00000, -0.42383) |
| H | (4b) (0.25000, 0.44890, -0.15423) |
| H | (4b) (0.25000, -0.07369, -0.25928) |
| $Cmcm$ (63) | $a = 3.67$Å, $b = 11.86$Å, $c = 7.19$Å |
| | $\alpha = \beta = \gamma = 90.00°$ |
| K | (4c) (0.00000, -0.30665, 0.25000) |
| Al | (4a) (0.00000, 0.00000, 0.00000) |
| H | (4b) (0.00000, 0.50000, 0.00000) |
| H | (8f) (0.00000, 0.14136, -0.00402) |
| H | (4c) (0.00000, 0.00829, 0.25000) |
| **Magnesium alanate $Mg(AlH_4)_2$** | |
| $P2_1$ (4) | $a = 4.51$Å, $b = 4.55$Å, $c = 9.98$Å |
| | $\alpha = 90.00°, \beta = 101.96°, \gamma = 90.00°$ |
| Mg | (2a) (0.29512, -0.02634, -0.40274) |
| Al | (2a) (0.24390, 0.22281, -0.00022) |
| Al | (2a) (-0.15399, 0.47331, -0.29219) |
| H | (2a) (0.38636, -0.31990, 0.29310) |
| H | (2a) (-0.42226, -0.36043, -0.42744) |
| H | (2a) (-0.05889, 0.39831, 0.03577) |
| H | (2a) (0.13407, 0.30705, -0.17280) |
| H | (2a) (-0.44962, 0.04055, -0.03447) |
| H | (2a) (0.33498, 0.13731, 0.17300) |
| H | (2a) (-0.08015, 0.26546, 0.29238) |

to be continued ..

**TABLE I – continued from previous page**

| | |
|---|---|
| H | (2a) (0.01015, -0.19229, 0.42758) |
| $P2$ (3) | $a = 4.48$Å, $b = 5.31$Å, $c = 4.41$Å |
| | $\alpha = 90.00°, \beta = 92.67°, \gamma = 90.00°$ |
| Mg | (1d) (0.50000, -0.33533, 0.50000) |
| Al | (1a) (0.00000, -0.09108, 0.00000) |
| Al | (1c) (0.50000, 0.21369, 0.00000) |
| H | (2e) (0.32816, -0.06011, -0.22224) |
| H | (2e) (0.33807, 0.41064, -0.24975) |
| H | (2e) (0.15455, -0.30170, 0.24011) |
| H | (2e) (0.18354, 0.15639, 0.19890) |
| $C2/m$ (12) | $a = 8.89$Å, $b = 10.86$Å, $c = 4.42$Å |
| | $\alpha = 90.00°, \beta = 92.03°, \gamma = 90.00°$ |
| Mg | (4h) (0.00000, -0.35319, 0.50000) |
| Al | (4i) (0.26981, 0.00000, 0.00411) |
| Al | (4g) (0.00000, -0.13584, 0.00000) |
| H | (8j) (0.08219, 0.23232, 0.24755) |
| H | (8j) (0.16431, 0.38456, -0.22268) |
| H | (4i) (-0.08071, 0.00000, -0.21114) |
| H | (4i) (0.40761, 0.00000, -0.26730) |
| H | (8j) (-0.33887, 0.39048, -0.19922) |
| **Calcium alanate $Ca(AlH_4)_2$** | |
| $P2_1/c$ (14) | $a = 4.16$Å, $b = 4.16$Å, $c = 11.95$Å |
| | $\alpha = 90.00°, \beta = 108.40°, \gamma = 90.00°$ |
| Ca | (2a) (0.00000, 0.00000, 0.00000) |
| Al | (4e) (-0.28230, 0.14675, -0.30741) |
| H | (4e) (-0.48587, 0.37669, -0.41016) |
| H | (4e) (-0.42854, 0.14663, 0.30279) |
| H | (4e) (0.02899, 0.04501, 0.19849) |
| H | (4e) (0.08832, 0.01889, 0.40979) |
| $C2$ (5) | $a = 12.06$Å, $b = 4.10$Å, $c = 4.19$Å |
| | $\alpha = 90.00°, \beta = 81.76°, \gamma = 90.00°$ |
| Ca | (2a) (0.00000, 0.25891, 0.00000) |
| Al | (4c) (0.30667, 0.43109, -0.28675) |
| H | (4c) (-0.41202, 0.25256, 0.11586) |
| H | (4c) (-0.30321, 0.15498, -0.40771) |
| H | (4c) (-0.09489, 0.18145, -0.48305) |
| H | (4c) (-0.19922, 0.22039, 0.04385) |
| $Pm$ (6) | $a = 6.56$Å, $b = 7.64$Å, $c = 4.24$Å |
| | $\alpha = 90.00°, \beta = 108.40°, \gamma = 90.00°$ |
| Ca | (1a) (-0.21687, 0.00000, 0.45419) |
| Ca | (1b) (0.49695, 0.50000, 0.30495) |
| Al | (2c) (0.31678, 0.17579, -0.41342) |
| Al | (2c) (-0.03929, 0.32428, -0.08756) |
| H | (2c) (-0.20211, -0.32774, -0.48443) |
| H | (2c) (0.11848, -0.16737, -0.21910) |
| H | (1a) (0.45169, 0.00000, -0.16278) |
| H | (2c) (0.44972, -0.34772, -0.19560) |
| H | (2c) (0.15901, 0.33247, 0.30057) |
| H | (2c) (-0.17261, 0.15243, -0.00059) |
| H | (2c) (0.48025, -0.17230, 0.34956) |
| H | (1a) (0.16273, 0.00000, 0.35438) |
| H | (1b) (-0.17406, 0.50000, 0.03291) |
| H | (1b) (0.11440, 0.50000, -0.16883) |
| **Strontium alanate $Sr(AlH_4)_2$** | |
| $Pm$ (6) | $a = 6.72$Å, $b = 7.81$Å, $c = 4.37$Å |
| | $\alpha = 90.00°, \beta = 72.05°, \gamma = 90.00°$ |
| Sr | (1a) (0.21662, 0.00000, 0.34191) |
| Sr | (1b) (-0.49047, 0.50000, 0.17763) |
| Al | (2c) (-0.31192, 0.17411, -0.27840) |
| Al | (2c) (0.03366, 0.32565, 0.05810) |
| H | (2c) (0.18921, -0.32914, 0.29460) |

to be continued ..

**TABLE I – continued from previous page**

| | |
|---|---|
| H | (2c) (-0.12429, -0.17298, 0.34016) |
| H | (1a) (-0.44681, 0.00000, -0.39065) |
| H | (2c) (-0.44381, -0.34081, -0.36133) |
| H | (2c) (-0.15378, 0.32725, -0.14631) |
| H | (2c) (0.16481, 0.15860, -0.14952) |
| H | (2c) (-0.46680, -0.17064, 0.10502) |
| H | (1a) (-0.15983, 0.00000, -0.20754) |
| H | (1b) (0.16982, 0.50000, -0.17830) |
| H | (1b) (-0.11881, 0.50000, 0.27395) |
| $P2_1/c$ (14) | $a = 10.74$Å, $b = 4.52$Å, $c = 12.07$Å |
| | $\alpha = 90.00°, \beta = 23.64°, \gamma = 90.00°$ |
| Sr | (2b) (0.50000, 0.00000, 0.00000) |
| Al | (4e) (0.24591, -0.41234, -0.00240) |
| H | (4e) (0.44015, 0.48321, -0.04678) |
| H | (4e) (0.48947, -0.40468, 0.30376) |
| H | (4e) (0.05630, -0.19912, -0.46170) |
| H | (4e) (-0.01740, 0.20644, -0.27913) |
| $P\bar{1}$ (2) | $a = 4.45$Å, $b = 5.86$Å, $c = 4.46$Å |
| | $\alpha = 82.96°, \beta = 93.91°, \gamma = 104.60°$ |
| Sr | (1h) (0.50000, 0.50000, 0.50000) |
| Al | (2i) (0.20564, -0.13595, 0.04876) |
| H | (2i) (-0.30539, 0.37303, 0.05150) |
| H | (2i) (-0.14144, -0.13990, -0.15458) |
| H | (2i) (0.42050, 0.05774, -0.24357) |
| H | (2i) (-0.05548, 0.28437, -0.37319) |
| **Reference (isolated) structure for strontium alanate $Sr(AlH_4)_2$** | |
| $P\bar{1}$ (2) | $a = 7.34$Å, $b = 6.61$Å, $c = 6.44$Å |
| | $\alpha = 116.83°, \beta = 77.81°, \gamma = 82.93°$ |
| Sr | (2i) (-0.22657, -0.43364, 0.33412) |
| Al | (2i) (0.26651, 0.11974, -0.04604) |
| Al | (2i) (0.25319, -0.26007, 0.35768) |
| H | (2i) (0.07338, -0.34867, 0.47080) |
| H | (2i) (0.19747, 0.02204, -0.48404) |
| H | (2i) (-0.28208, 0.36532, -0.06979) |
| H | (2i) (-0.07343, -0.30874, 0.00379) |
| H | (2i) (0.22755, -0.13838, -0.16011) |
| H | (2i) (0.42972, 0.15590, -0.23470) |
| H | (2i) (0.31926, 0.19379, 0.20751) |
| H | (2i) (0.42586, -0.40056, 0.40593) |

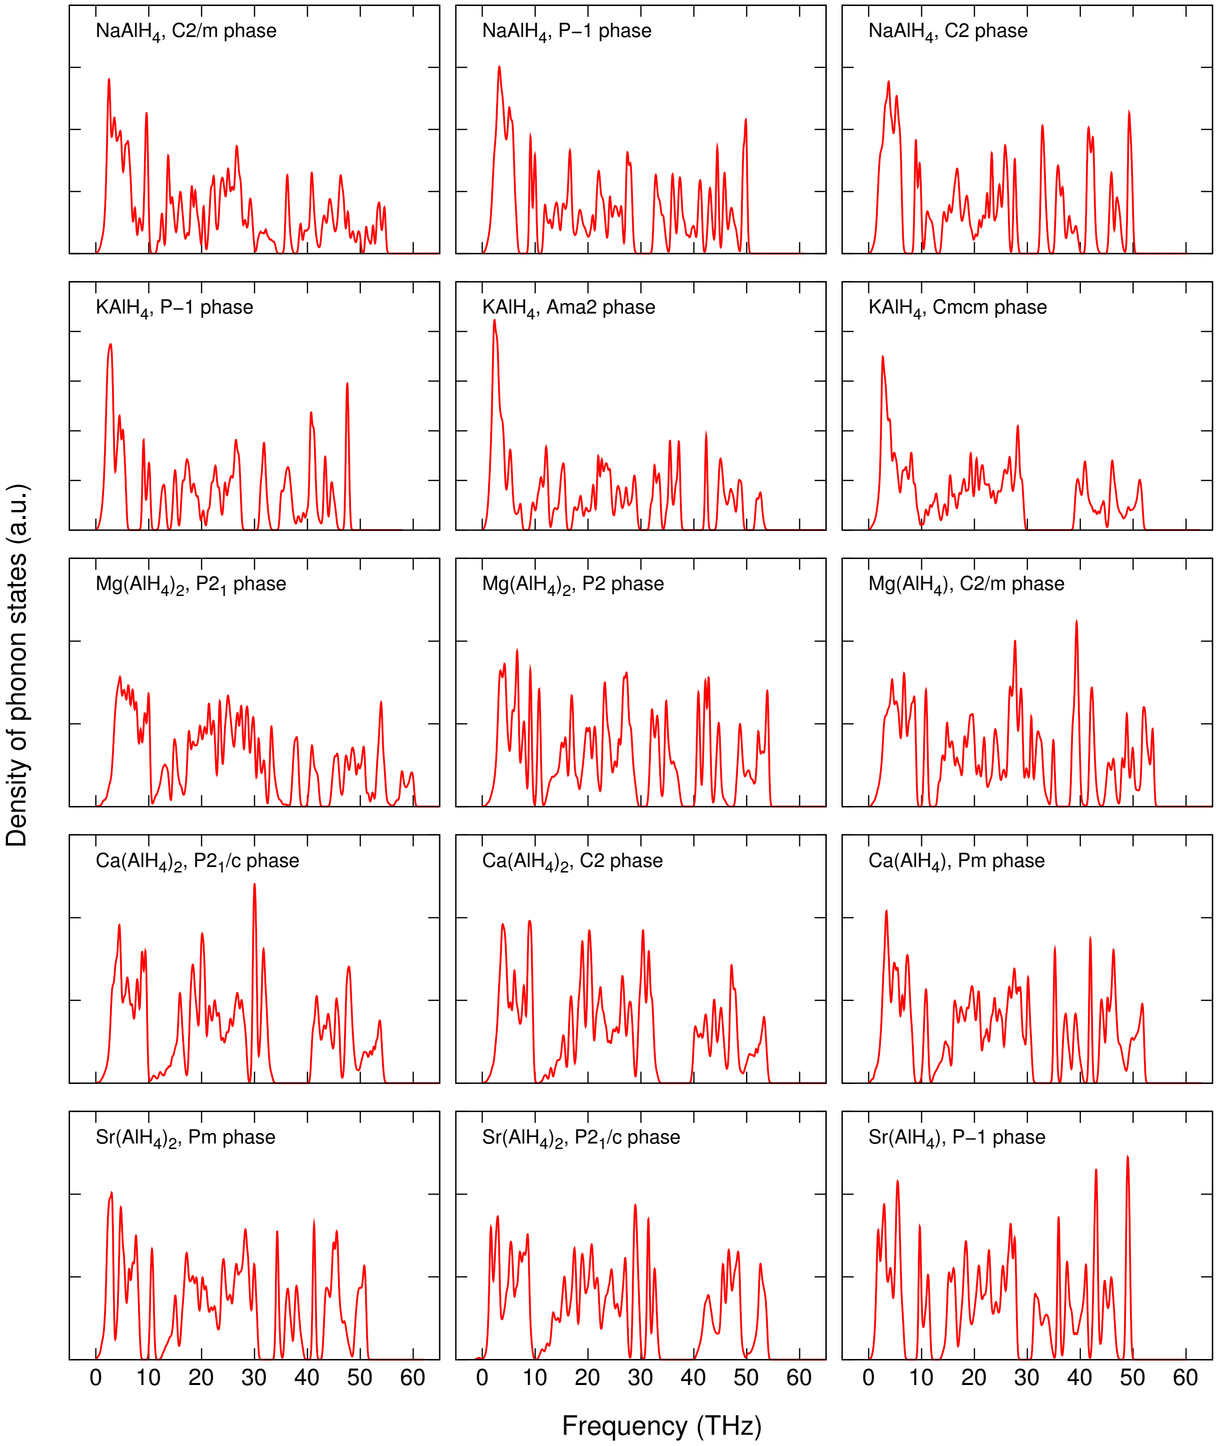


FIG. 1. (Color online) Densities of phonon states of three most stable polymeric phases of $NaAlH_4$, $KAlH_4$, $Mg(AlH_4)_2$, $Ca(AlH_4)_2$, and $Sr(AlH_4)_2$.

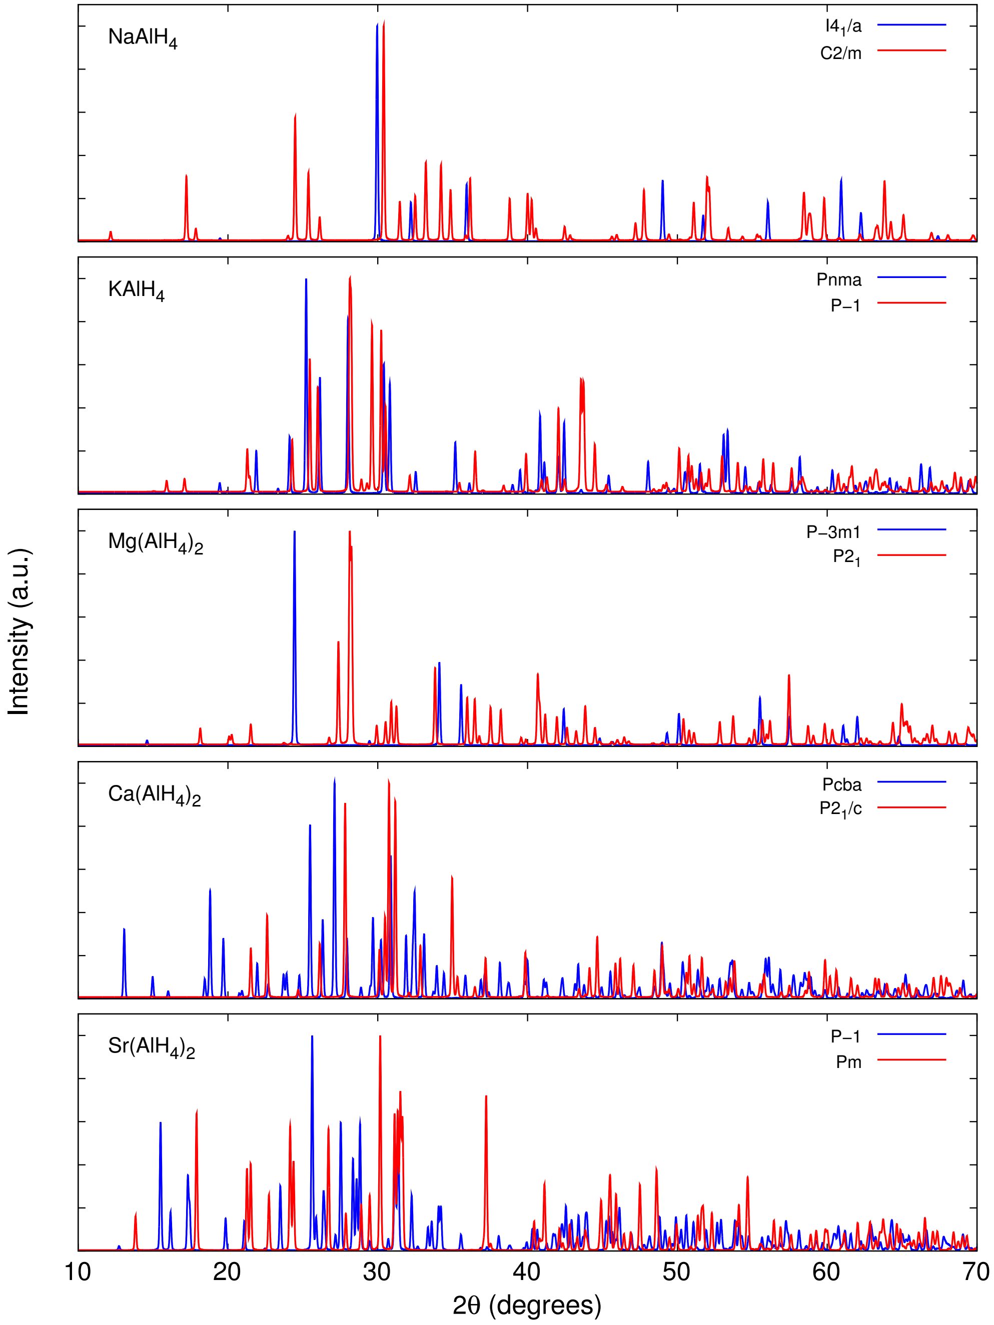


FIG. 2. (Color online) Simulated X-ray diffraction spectra of the most stable polymeric phases in a comparison with the corresponding reference isolated phases of $NaAlH_4$, $KAlH_4$, $Mg(AlH_4)_2$, $Ca(AlH_4)_2$, and $Sr(AlH_4)_2$.
